# Supplementary material for: PhysGen3D: Crafting a Miniature Interactive World from a Single Image
Source: arXiv:2503.20746 source file (2025-03-26)
Supplement: Supplementary file 1 [file control.tex]

\begin{figure*}[t]
    \centering
    \includegraphics[width=\linewidth]{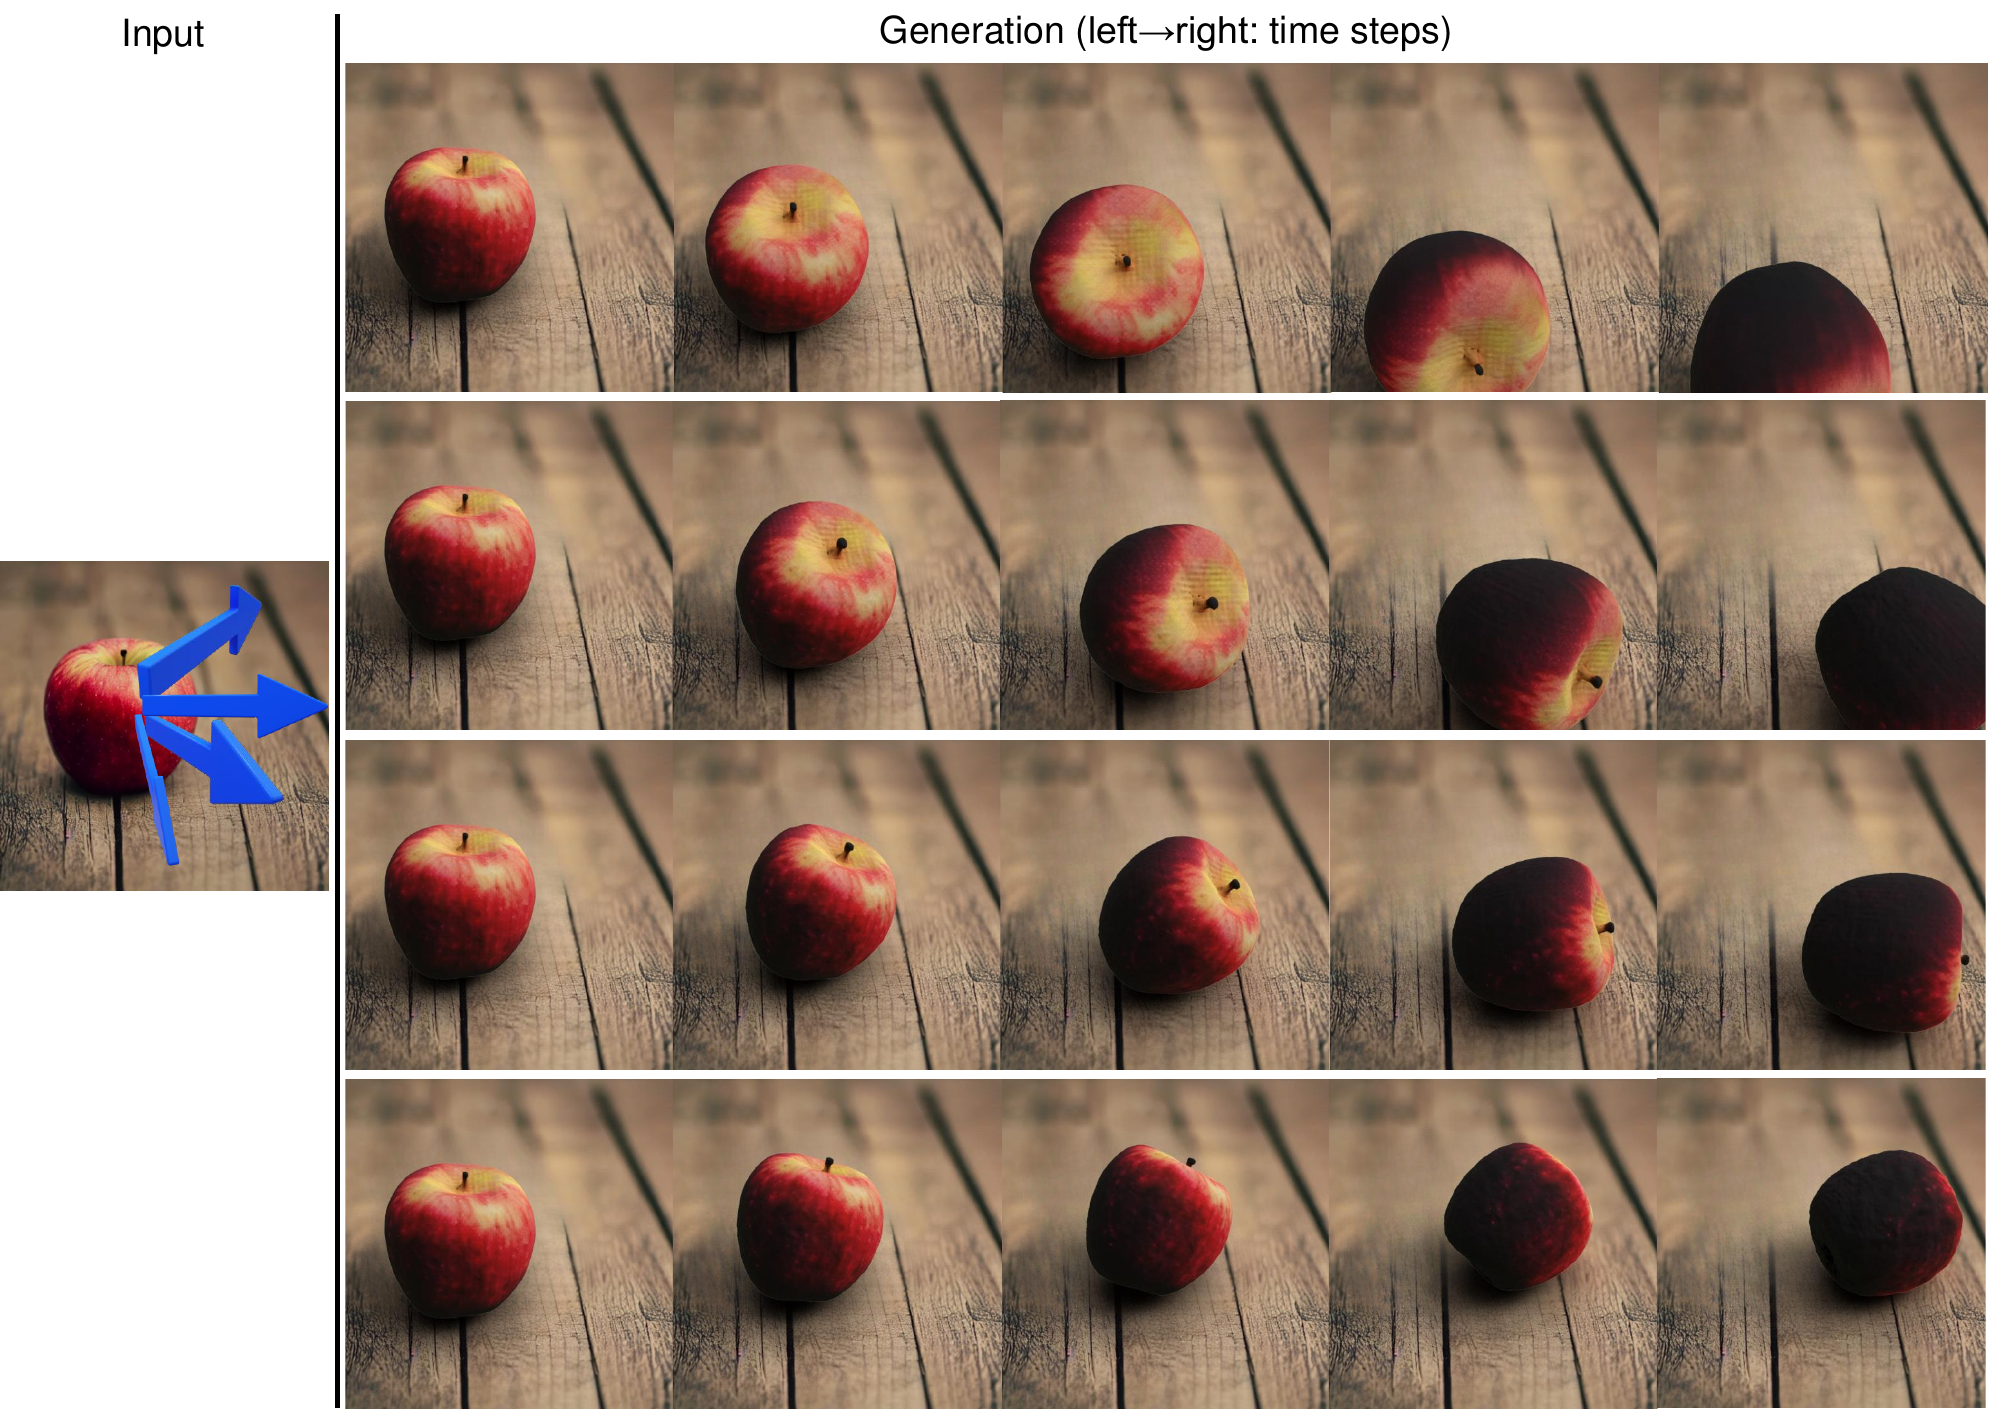}
    \caption{\small
    \textbf{More Results about dynamics control.} We generate a series of videos from the same input image, each with a different initial velocity—maintaining the same speed but varying the direction. This demonstrates our method's ability to precisely control motion details.
    }
    \label{fig:control}
    \vspace{-5pt}
\end{figure*}
